# Supplementary material for: A Hamilton-Jacobi Reachability-Based Framework for Predicting and Analyzing Human Motion for Safe Planning
Source: arXiv:1910.13369 source file (2020-04-05)
Supplement: Supplementary file 1 [file supplementary.tex]

\section{Supplementary Material}

\subsection{Dynamics of $\ptparam$} \label{subsec:beta_dynamics}
